# Supplementary material for: Ensemble Data Assimilation for Particle-based Methods
Source: arXiv:2410.19525 source file (2024-12-08)
Supplement: Supplementary file 1 [file appendix.tex]

% !TEX root = main.tex
\section{Stochastic Ensemble Kalman Filter}\label{appendix:enkf}
We define the matrix of states and the matrix of anomalies $\mstate^f = [\statebis^1 | \dots | \statebis^N]$, $\annomX$ whose columns are the member states and the normalized anomalies:
\begin{equation*}
    \annomX = \frac{1}{\sqrt{N - 1}}(\mstate^f - \overline{\statebis}^f \bm{1}^T),
\end{equation*}where $\bm{1} \in \mathbb{R}^N$ is a vector of one.

Similarly, the matrix of observation and observation anomalies are $\mathcal Y^f = [\mathcal{H}(\statebis_1^f) | \dots | \mathcal{H}(\statebis_N^f)]$ and $\annomY$ where columns are
\begin{equation*}
    \annomY = \frac{1}{\sqrt{N - 1}} \left(\mathcal Y - \overline{\obs} \bm{1}^T \right) \quad \text{with} \quad \overline{\obs} = \frac{1}{N} \sum_{j=1}^{N} \mathcal{H}(\statebis_j^f).
\end{equation*}

Ensemble is used to defined covariance matrices and $\tilde{\bm{K}}$ the Kalman gain
\begin{eqnarray*}
    \Cov \bm H^T &\simeq& \frac{1}{N - 1} \sum_{i = 1}^{N} {(\statebis_i^f - \overline{\statebis}^f)} {\left[ \mathcal{H}(\statebis_i^f) - \overline{\bm{y}}\right]}^T = \annomX \annomY^T, \\
    \bm H \Cov \bm H^T &\simeq& \frac{1}{N -1} \sum_{i = 1}^{N}\left[ \mathcal{H}(\statebis_i^f) - \overline{\bm{y}}\right] {\left[ \mathcal{H}(\statebis_i^f) - \overline{\bm{y}}\right]}^T = \annomY \annomY^T,\\
    \tilde{\bm{K}} &=& \Cov \bm H^T{(\bm H \Cov \bm H^T + \bm R)}^{-1} = \annomX \annomY^T {(\annomY \annomY^T + \bm R)}^{-1}.
\end{eqnarray*}

The forecast is then updated to a posterior ensemble $\left\{\statebis_i^a\right\}_{i=1}^{N}$ such that
\begin{equation}~\label{enkf_formula}
    \mstate^a = \mstate^f + \tilde{\bm{K}} ( \mdata - \mpred),
\end{equation}where ${[\mdata]}_i = \bm d + \bm{\varepsilon}_i$ is the perturbed observation with $\bm{\varepsilon}_i \sim \mathcal{N}(\bm{0}, \bm R) $, $\tilde{\bm{K}}$ the ensemble Kalman gain matrix and $( \mdata - \mpred)$ the innovation term.
The forecast step is then applied to the analyzed ensemble until the next observation.
Based on this formulation, we can deduce a correction formula only based on the member's predictions and observations.

We can rewrite the classical update formula using the previous anomaly matrices.
\begin{equation*}
    \mstate^a = \mstate^f + \annomX \annomY^T {({\annomY \annomY^T + \bm R})}^{-1}(\mdata - \mpred)
\end{equation*}

We reformulate the correction term by remarking that $ \bm{1}^T  \annomY^T = \bm{0}$. We define $\Fcorr$, the correction matrix that gives the update in terms of linear combinations of the forward states
\begin{equation*}
    \mstate^a = \mstate^f + \mstate^f \Fcorr, \quad \Fcorr = \frac{1}{\sqrt{N - 1}}\annomY^T {(\annomY \annomY^T + \bm R)}^{-1}(\mdata - \mpred).
\end{equation*}

using the Sherman-Morrison-Woodbury formula we obtain
\begin{equation*}
    \Fcorr = \frac{1}{\sqrt{N - 1}} {(\bm I_N + \annomY^T\bm R^{-1}\annomY)}^{-1}\annomY^T \bm R^{-1} (\mdata - \mpred).
\end{equation*}
